# Supplementary material for: Coherence in Molecular Photoionization
Source: arXiv:1705.06276 source file (2017-05-17)
Supplement: Supplementary file 1 [file AyusoJPCA2015-SI.pdf]

# Vibrationally Resolved B 1s Photoionization Cross Section of $BF_3$
# – Supporting Information –

D. Ayuso,[†] M. Kimura,[‡] K. Kooser,[¶] M. Patanen,[§] E. Plésiat,[†] L. Argenti,[†] S. Mondal,[‡] O. Travnikova,[§] K. Sakai,[‡] A. Palacios,[†] E. Kukk,[¶] P. Decleva,[‖] K. Ueda,[‡] F. Martín,[*,†,#] and C. Miron[*,§,@]

*Departamento de Química, Módulo 13, Universidad Autónoma de Madrid, 28049 Madrid, Spain, Institute of Multidisciplinary Research for Advanced Materials, Tohoku University, Sendai 980-8577, Japan, Department of Physics and Astronomy, University of Turku, 20014 Turku, Finland, Synchrotron SOLEIL, L'Orme des Merisiers, Saint-Aubin, BP 48, 91192 Gif-sur-Yvette Cedex, France, and Dipartimento di Scienze Chimiche e Farmaceutiche, Universita di Trieste, Via L. Giorgieri 1, I-34127 Trieste, Italy and CNR–Istituto Officina dei Materiali, 34127 Trieste, Italy*

E-mail: fernando.martin@uam.es; catalin.miron@synchrotron-soleil.fr

[*]To whom correspondence should be addressed

[†]Departamento de Química, Módulo 13, Universidad Autónoma de Madrid, 28049 Madrid, Spain

[‡]Institute of Multidisciplinary Research for Advanced Materials, Tohoku University, Sendai 980-8577, Japan

[¶]Department of Physics and Astronomy, University of Turku, 20014 Turku, Finland

[§]Synchrotron SOLEIL, L'Orme des Merisiers, Saint-Aubin, BP 48, 91192 Gif-sur-Yvette Cedex, France

[‖]Dipartimento di Scienze Chimiche e Farmaceutiche, Universita di Trieste, Via L. Giorgieri 1, I-34127 Trieste, Italy and CNR–Istituto Officina dei Materiali, 34127 Trieste, Italy

[⊥]Instituto Madrileño de Estudios Avanzados en Nanociencia (IMDEA-Nanociencia), Cantoblanco, 28049 Madrid, Spain

[#]Condensed Matter Physics Center (IFIMAC), Universidad Autónoma de Madrid, 28049 Madrid, Spain

[@]Extreme Light Infrastructure - Nuclear Physics (ELI-NP), "Horia Hulubei" National Institute for Physics

## Generalized $\nu$–ratio, $G$ factor

In the study of C 1s photoionization cross section of $CH_4$, Plésiat *et al.* (see Ref. 37 of the main manuscript) presented a simple analytical model based on a Born approximation that can be applied to B 1s cross section of $BF_3$ as well. This model gives a straightforward physical picture of the photoelectron scattering and provides a clear parametrization for the relative variation of the height of an individual vibrational peak observed in the photoionization spectrum. More specifically, according to the model, the intensity $I_\nu(E)$ of any given peak in the totally symmetric stretching mode has the following form:

$$I_\nu(E) = FC_\nu[I^0(E) + I^1(E) + \nu I^2(E)] \tag{1}$$

where $FC_\nu$ are energy-independent Franck-Condon parameters, $I^0(E)$ is a smooth, atomic-like photoionization cross section, $I^1(E)$ is an oscillating term, which is much smaller than $I^0(E)$ and which does not depend on $\nu$, i.e., an oscillation of the total cross section which would be present even for a completely rigid molecule. $I^2(E)$ is a second oscillating term which is one order of magnitude smaller than $I^1(E)$ and is multiplied by the vibrational quantum number $\nu$ of the parent ion. This term, $\nu I^2(E)$, is responsible for the oscillation in the vibrationally-resolved cross section ratio.

We define the ratio $R_\nu(E)$ as an intensity ratio of a given vibrational peak $I_\nu(E)$ to the total cross section at energy $E$, $I_{tot}(E) = \sum_\nu I_\nu(E)$:

$$R_\nu(E) = FC_\nu[1 + (\nu - \nu_{av})J(E)] \tag{2}$$

where $\nu_{av} = \sum_\nu FC_\nu \nu$ is the average vibrational quantum number of the parent ion, and $J(E) = I^2(E)/[I^0(E) + I^1(E) + I^2(E)]$.

If $I^0(E)$ is much larger than $I^1(E)$ and $I^2(E)$, then the function $J(E)$ is an oscillatory

and Nuclear Engineering, 30 Reactorului Street, RO-077125 Măgurele, Jud. Ilfov, Romania

function similar to $j_1(2kR)$ (see Ref. 37 of the main manuscript).

From the Eq. 2 we can see that the relative intensities can be approximated with a Taylor expansion with respect to $(\nu - \nu_{av})$ truncated to the first order. This parametrization assumes that the deviations from Franck-Condon are small and smooth across the photoelectron signal, which is a reasonable assumption outside the resonant energies. Thus, the equation 2 provides a way to describe the fluctuation of the whole Franck-Condon envelope with one parameter during the fitting process of each spectrum. From a practical point of view it turned out to be better to modify Eq. 2 and express the FC parameters as a function of the actual ratios $R_\nu(E_0)$ at a given reference energy $E_0$:

$$FC_\nu = R_\nu(E_0)/[1 + (\nu - \nu_{av})J(E_0)]. \quad (3)$$

Then, Eq. 2 can be rearranged as

$$R_\nu(E) = R_\nu(E_0)\{1 + (\nu - \nu_{av})[J(E) - J(E_0)]/[1 + (\nu - \nu_{av})J(E_0)]\} \quad (4)$$

At relatively high energy, $J(E)$ is expected to be small. Accurate theoretical predictions estimate an amplitude below 0.01 above E=100 eV. To a first approximation, therefore, If $(\nu - \nu_{av})$ $J(E_0)$ is negligible when compared to 1, which allows one to write

$$R_\nu(E) \sim R_\nu(E_0)[1 + (\nu - \nu_{av})(J(E) - J(E_0))] \quad (5)$$

This expression provides a way to extract a single value $G(E) = J(E) - J(E_0)$ representing the oscillations of the spectrum at a given energy $E$ with respect to a chosen $E_0$ value. $E_0$ was chosen arbitrarily to be the point at 24 eV above threshold. This method ensures much better statistics for the experiment since all the individual TSSM peaks of a given spectrum contribute to the same fitting parameter.

To compare with the experimental data, $G(E)$ can be obtained for the static-exchange

DFT calculations from $J(E)$ by inverting Eq. 2:

$$J(E;\nu) = [R_\nu(E)/FC_\nu - 1]/(\nu - \nu_{av}). \quad (6)$$

Finally, a weighted average of all the different $J(E,\nu)$ was taken to obtain the $G$ factor from the calculations

$$G_{th}(E) = \sum_\nu J(E;\nu) FC_\nu. \quad (7)$$

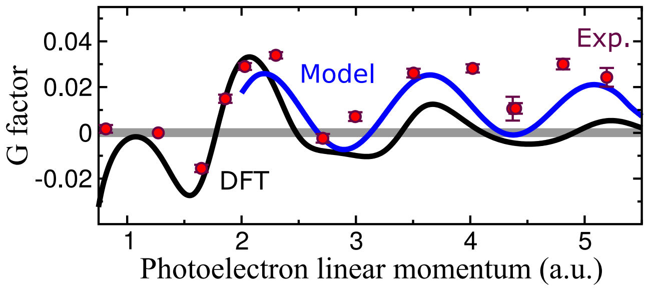


Figure 1: Generalized $\nu$-ratio ($G$ factor) for $BF_3$ as a function of photoelectron momentum. Circles with error bars: experimental results including statistical errors. Black line: results from the static-exchange DFT calculations. Blue line: results of the simple analytical model explained in the text.

Figure 1 presents the comparison between the experimental and theoretical generalized ratio $G(E)$. The agreement of the experimental data with the theoretical predictions is quite convincing (note that the second point is the one chosen as a reference). The Born approximation based scattering model catches nicely the three maxima between 2–5 a.u., but cannot be used to describe the data at very low electron momenta, where the static-exchange DFT calculations give a very good agreement with the experimental data. As already discussed in Ref. 15 of the main manuscript, the good agreement with the scattering model and the experiment at high energies proves the origin of these oscillations to be photoelectron diffraction.
