# Supplementary material for: Coherence in Molecular Photoionization
Source: arXiv:1705.06276 source file (2017-05-17)
Supplement: Supplementary file 2 [file CalegariScience2014-SM.pdf]

www.sciencemag.org/content/346/6207/336/suppl/DC1

# Supplementary Material for

## Ultrafast electron dynamics in phenylalanine initiated by attosecond pulses

F. Calegari, D. Ayuso, A. Trabattoni, L. Belshaw, S. De Camillis, S. Anumula, F. Frassetto, L. Poletto, A. Palacios, P. Decleva, J. Greenwood, F. Martín,* M. Nisoli*

*Corresponding author. E-mail: fernando.martin@uam.es (F.M.); mauro.nisoli@polimi.it (M.N.)

Published 17 October 2014, *Science* **346**, 336 (2014)
DOI: 10.1126/science.1254061

**This PDF file includes:**

Materials and Methods

Supplementary Text

Figs. S1 to S11

Tables S1 and S2

Full Reference List

**Other Supplementary Material for this manuscript includes the following:**
(available at www.sciencemag.org/content/346/6207/336/suppl/DC1)

Movie S1

## Materials and Methods

Experimental setup

For the experiments a Ti:sapphire laser system was used (Femtopower PRO HE CEP, Femtolasers) delivering 6-mJ pulses, with 25-fs duration and 1-kHz repetition rate. The carrier-envelope phase (CEP) was stabilized by two feedback loops: a fast loop acting on the oscillator and a slow loop acting on a glass wedge placed in the stretcher before the preamplifier. The pulses used for the experiments present a residual CEP fluctuation of ~200 mrad (rms), measured in-loop with a *f*-2*f* interferometer using an integration time of 1 ms. We have first compressed the pulses using a hollow-fiber (*32*) with pressure gradient (*33*) and a broadband chirped-mirror dispersive delay line. We used a 1-m-long hollow fiber with an inner diameter of 320 µm, filled with helium: the pressure at the input of the fiber was kept to <5 mbar and 2 bar at the output. The beam position at the input of the hollow fiber was actively stabilized. A pulse energy of 3.3 mJ was obtained at the output with no gas in the fibre, and 2.3 mJ with gas. After 8 reflections on the chirped mirrors, pulses as short as 4 fs were achieved. The pulse duration was measured by using a single-shot Self-Referenced Spectral Interferometry method (*34*) implemented with Cross-Polarized Wave (XPW).

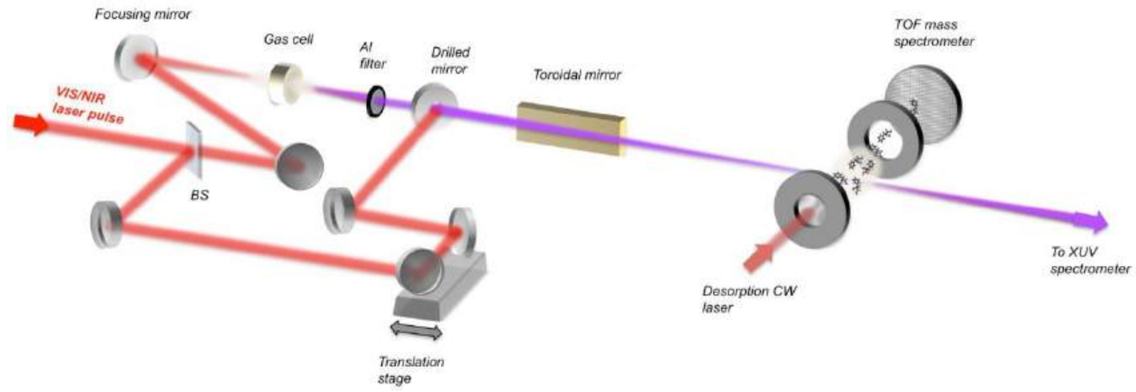


**Fig. S1.**
**Pump-probe experimental setup.** Experimental setup for the pump-probe measurements. BS is a broadband beam-splitter with 30% reflection; TOF mass spectrometer is a time of flight mass spectrometer. The focusing mirror has a 1-m radius of curvature.

The experimental setup used for the pump-probe measurements is shown in Fig. S1. The visible/near infrared (VIS/NIR) beam was divided into two parts using a beam splitter with 30% reflection. The transmitted portion of the beam was focused by a 1-m radius of curvature mirror into a 3-mm-thick cell filled with xenon at static pressure to produce extreme ultraviolet (XUV) radiation by high-order harmonic generation (HHG). Isolated attosecond pulses, with energy in the nanojoule range, were produced by employing the ionization gating technique (*35*). A 100-nm-thick aluminium filter was used to filter out the fundamental radiation and the low order harmonics. An indium foil has been also used in a few measurements described in the text. The temporal duration of

the XUV pulses (290±20 as) was measured by using the Frequency Resolved Optical Gating for Complete Reconstruction of Attosecond Bursts (FROG CRAB) technique (*36-37*). The remaining part of the VIS/NIR beam was collinearly recombined with the XUV beam by using a mirror with a central hole. The temporal delay between VIS/NIR and XUV pulses was adjusted with attosecond resolution by using a piezoelectric translation stage. The pump and probe pulses were collinearly focused into the mass spectrometer by using a gold-coated toroidal mirror, with unit magnification, which provided an almost aberration-free image of the XUV source with negligible temporal smearing of the attosecond pulses (*38*). The peak intensity of the VIS/NIR probe pulse in the sample was about $5\times10^{12}$ W/cm$^2$. The spectrum of the XUV radiation was measured by using a high-resolution flat-field soft x-ray spectrometer consisting of a grating, followed by a phosphor screen, and a charge-coupled device (CCD) camera (*38*).

## Molecular Target Preparation

For the experiments, 99% DL-Phenylalanine was acquired from Sigma-Aldrich and used without further purification. It was rubbed directly onto the surface of a 301 stainless steel foil of 10-μm thickness and 12-mm diameter and then clamped into the repeller electrode of a time of flight mass spectrometer (*23*). The distance from the foil, and hence the sample, to the focal point of the ionizing laser pulses was approximately 3 mm. To evaporate the sample, the reverse side of the foil was irradiated with a CW diode laser operating at a wavelength of 960 nm, with a spot diameter of 6 mm and power in the range 0.3 – 0.4 W.

The temperature of the sample was estimated by assuming equilibrium heat conduction along the foil to the repeller electrode (which acts as a room temperature heat sink) and that 30% of the incident radiation was absorbed by the foil at this wavelength (*39*). Radiative heat losses were negligible for the calculated temperatures. For the lowest laser power used, the temperature at the centre of the foil was estimated to be 430 K and about 410 K at a radius of 2 mm. As the sample depleted, to increase the evaporation at greater distances from the center, the diode laser power was increased to maintain a constant target gas density. While the evaporated target molecules were relatively hot, no fragmentation of the molecules was expected prior to interaction with the ionizing pulses. It was observed that using only the 4 fs VIS/NIR pulses to ionize the molecules produced predominantly parent ions in the mass spectrum. In other experiments using an even softer ionization method (near threshold single photon ionization), parent phenylalanine ions constituted more than 90% of the mass spectrum for a molecular temperature of 423 K (*40*). Therefore, we can conclude that the observed ultrafast dynamics can be attributed to the parent phenylalanine cation and that loss of the carboxyl group to form the immonium dications occurs after interaction with the pump and probe pulses.

## Fitting of the oscillations in the yield of immonium dication

The pump-probe measurement shown in Fig. 2A, acquired in the case of 3-fs temporal step for the delay between pump and probe pulses, has been fitted by the convolution, $F(t)$, of a Gaussian pulse of 4-fs full-width at half maximum (FWHM) corresponding to probe pulse duration, with the following function:

$$R(t) = A(e^{-t/\tau_1} - e^{-t/\tau_2}) \quad (1)$$

where $\tau_1$ = 10±2 fs and $\tau_2$ = 25±2 fs. In order to fit the temporal evolution of the oscillations in the yield of the doubly-charged immonium fragment, we have first subtracted the fitting curve $F(t)$ (assuming $\tau_1$ = 10 fs and $\tau_2$ = 25 fs)from the experimental data acquired in the case of 0.5-fs delay-steps.

At short pump-probe delays ($t$ < 10 fs) Fourier analysis shows the presence of two main frequency components around 0.14 PHz and 0.3 PHz, as displayed in the spectrogram of Fig. 3A. Therefore, the experimental data have been fitted by the sum of two sinusoidal functions:

$$S(t) = A_1 \sin(2\pi\nu_1 t + \phi_1) + A_2 \sin(2\pi\nu_2 t + \phi_2) \quad (2)$$

The curve has been calculated by using the fitting tool of Matlab R2011a with a confidence level for the bounds of 95%. The result is displayed in Fig. S2. The calculated frequencies are: 0.14 PHz (lower and upper confidence bounds: 0.12 PHz and 0.158 PHz, respectively) and 0.293 PHz (lower and upper confidence bounds: 0.281 PHz and 0.304 PHz, respectively). The total deviation is 0.0063 PHz and the root-mean-square deviation is 0.0148 PHz.

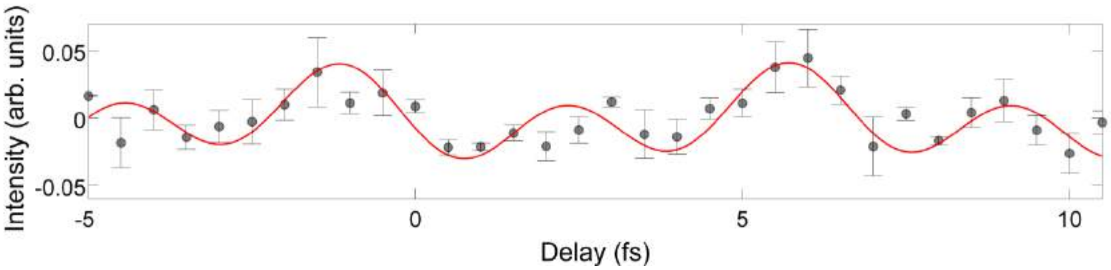


**Fig. S2**

**Fitting curve: short pump-probe delays ($t$ < 10 fs).** Dots correspond to the difference between the experimental data and the exponential fitting curve $F(t)$. Error bars show the standard error of the results of four measurements. Red curve is the corresponding fitting curve calculated considering the sum of two sinusoidal functions of frequencies 0.14 PHz ($A_1$ = 0.016, $\phi_1$ = 2.88 rad) and 0.293 PHz ($A_2$ = 0.025, $\phi_2$ = 3.62 rad).

In the delay range between 10 fs and 40 fs a strong and broad peak around 0.24 PHz is visible in the spectrogram of Fig. 3A, with a spectral width which slightly increases upon increasing the pump-probe delay. We have first fitted the experimental data by using a single sinusoidal function. The result is shown in Fig. 2C. The calculated frequency is 0.234 PHz, with lower and upper confidence bounds of 0.229 PHz and 0.238 PHz, respectively. The total deviation is 0.0069 PHz and the root-mean-square deviation is 0.0119 PHz. The amplitude and phase of the fitting curve are $A$ = 0.022 and $\phi$ = 1.75 rad, respectively.

The same data can be also fitted by the sum of two sinusoidal functions. The result is displayed in Fig. S3. The resulting frequencies are: 0.234 PHz (lower and upper confidence bounds: 0.229 PHz and 0.239 PHz, respectively) and 0.292 PHz (lower and upper confidence bounds: 0.277 PHz and 0.307 PHz, respectively). The total deviation of

0.0059 PHz and the root-mean-square deviation of 0.0113 PHz are slightly reduced compared to the single-frequency fitting.

Figure S4 shows the experimental data, after subtraction of the fitting curve $F(t)$, in the whole temporal region of the pump-probe measurement. The fitting curve displayed in the figure is the composition of the curves shown in Fig. S2 and S3.

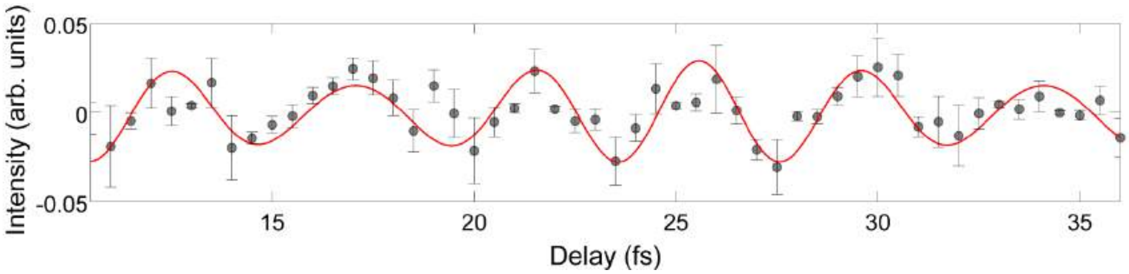


**Fig. S3**
**Fitting curve: delay range between 10 fs and 40 fs.** Dots correspond to the difference between the experimental data and the exponential fitting curve $F(t)$. Error bars show the standard error of the results of four measurements. Red curve is the corresponding fitting curve calculated considering the sum of two sinusoidal functions of frequencies 0.234 PHz ($A_1$ = 0.022, $\phi_1$ = 1.61 rad) and 0.292 PHz ($A_2$ = 0.007, $\phi_2$ = 4.88 rad).

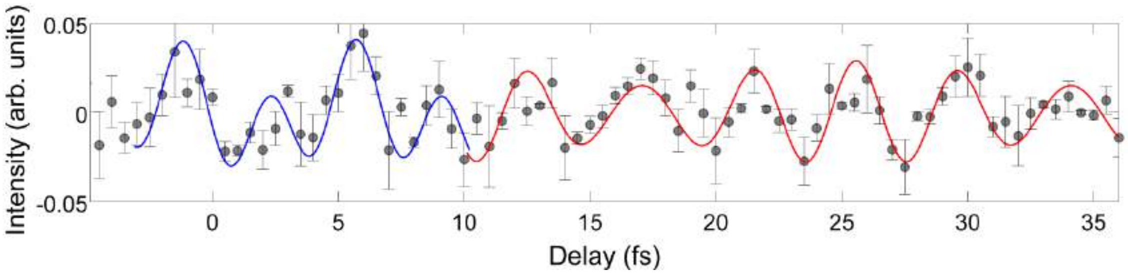


**Fig. S4**
**Fitting curve: whole delay range.** Dots correspond to the difference between the experimental data and the exponential fitting curve $F(t)$. Error bars show the standard error of the results of four measurements. Blue curve is the fitting curve shown in Fig. S2, red curve is the fitting curve shown in Fig. S3.

<u>Theoretical method</u>

As the XUV pulse is weak, we use time-dependent first-order perturbation theory to evaluate the ionization amplitudes at the end of the pulse $t = T$:

$$c_{\alpha\varepsilon l}(T) = -i\left\langle \Psi_{\alpha l}(\varepsilon,\vec{r})\,|\vec{e}\cdot\vec{r}\,|\,\Psi_0(\vec{r})\right\rangle \int_{-\infty}^{T} E(t)\, e^{i(E_\alpha+\varepsilon-E_0)t}dt \qquad (3)$$

where $\Psi_0$ is the all-electron (hereafter called $N$-electron) ground state of phenylalanine with energy $E_0$, $\Psi_{\alpha l}(\varepsilon)$ is the $N$-electron continuum state that describes a photoelectron ejected from the $\alpha$ molecular orbital with kinetic energy $\varepsilon$ and angular quantum number $l$ (for simplicity in the notation, we have omitted the $m$ quantum number), $E_\alpha$ is the corresponding cationic energy and $E(t)$ is the electric field associated with the XUV pulse polarized along the $\vec{e}$ direction. This electric field is derived from the experimental measurements. The $\Psi_0$ and $\Psi_{\alpha l}(\varepsilon)$ wave functions have been evaluated in the framework

of the fixed-nuclei approximation by using the static-exchange density functional theory (DFT) and the LB94 functional for exchange and correlation (see reference (*28*)) . A more accurate description of the corresponding energies has been obtained by using a local density approximation that includes the self-interaction correction term that ensures that the ionized electron sees the correct asymptotic charge. The electronic Kohn-Sham equations were solved by expanding the wave functions in a basis of multicentric B-spline functions. The static-exchange DFT method has been successfully used to study photoionization of a large number of diatomic and polyatomic molecules [see, e.g., (*28-30, 41-50*) and references therein].

Neglecting the interaction of the photoelectron with the remaining ($N$-1)-electron cation, the electronic density of the latter is given by (*51, 52*):

$$\rho_{\text{ion}}(\vec{r},t) = \sum_{\alpha}\Big(\sum_{\substack{\alpha' \\ \alpha'\neq\alpha}} \gamma^{(\text{ion})}_{\alpha'\alpha'}\Big)\ \varphi^2_{\alpha}(\vec{r}) - \sum_{\substack{\alpha\alpha' \\ \alpha'\neq\alpha}} \gamma^{(\text{ion})}_{\alpha\alpha'}\ e^{i(E_{\alpha'}-E_{\alpha})t}\varphi_{\alpha}(\vec{r})\,\varphi_{\alpha'}(\vec{r}) \qquad (4)$$

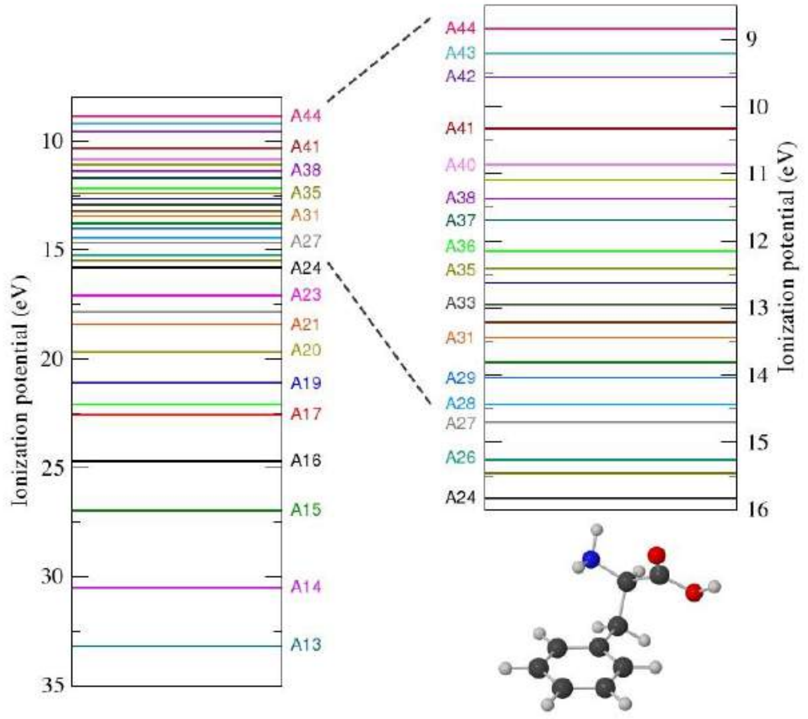


**Fig. S5**.

**Ionization potentials.** Ionization potentials for the most abundant conformer of the phenylalanine molecule obtained from static-exchange DFT-LDA calculations. The labels "An" denote the molecular orbital from which the electron is removed.

where $\varphi_{\alpha}(\vec{r})$ is the $\alpha$ molecular orbital and $\gamma^{(\text{ion})}_{\alpha\alpha'}$ is the reduced density matrix element defined as :

$$\gamma^{(\text{ion})}_{\alpha\alpha'} = \sum_{l}\int c_{\alpha l}(\varepsilon)\,c^{*}_{\alpha' l}(\varepsilon)\,d\varepsilon \qquad (5)$$

The hole density is given by the difference between the electronic density of the neutral molecule, which does not depend on time, and the electronic density of the cation:

$$\rho_{\text{hole}}(\vec{r},t) = \rho_{\text{neutral}}(\vec{r}) - \rho_{\text{ion}}(\vec{r},t) = \sum_{\alpha}\Big(1 - \sum_{\substack{\alpha' \\ \alpha'\neq\alpha}} \gamma^{(\text{ion})}_{\alpha'\alpha'}\Big)\, \varphi^2_{\alpha}(\vec{r}) + \sum_{\substack{\alpha\alpha' \\ \alpha'\neq\alpha}} \gamma^{(\text{ion})}_{\alpha\alpha'}\, e^{i(E_{\alpha'}-E_{\alpha})t} \varphi_{\alpha}(\vec{r})\, \varphi_{\alpha'}(\vec{r}) \tag{6}$$

where

$$\rho_{\text{neutral}}(\vec{r}) = \sum_{\alpha} \varphi^2_{\alpha}(\vec{r}) \tag{7}$$

**Supplementary Text**

Photoionization cross sections

Figure S5 shows the ionization energies of all open channels for the most abundant (according to Ref. (*27*)) conformer of phenylalanine. These energies are approximately given by the Kohn-Sham orbital energies resulting from the static-exchange DFT calculations. The blow-up shows the ionization energies for the highest channels.

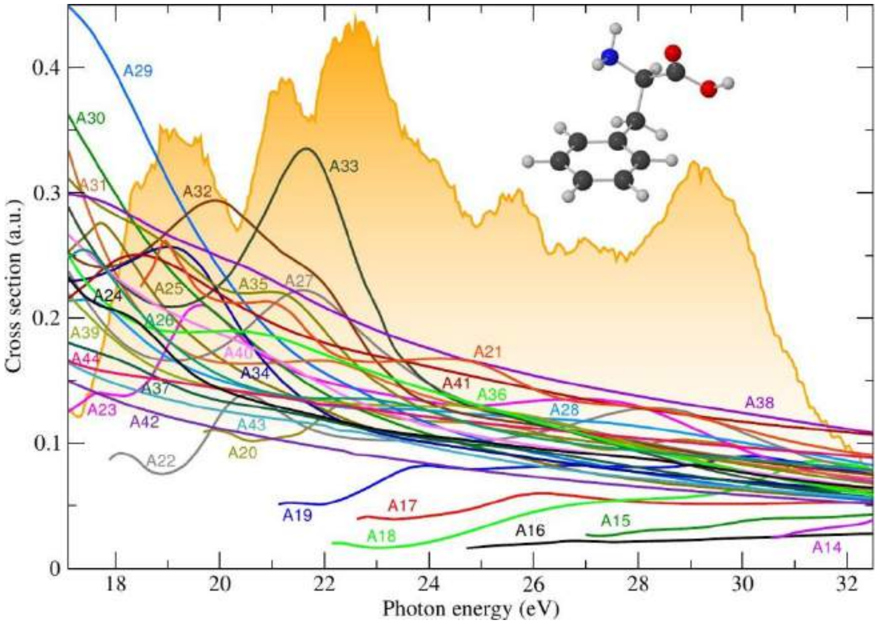


**Fig. S6.**

**Photoionization cross sections and spectrum of the attosecond pump pulse.**

Photoionization cross sections of the phenylalanine molecule from different molecular orbitals provided by the static-exchange DFT method. Numbers and colors denote the same molecular orbitals as in Fig. S5. The frequency spectrum of the attosecond pulse used in the experiment and in the calculations of the transition amplitudes leading to the coherent superposition of the one-hole states is represented by a thick orange curve lying over a shaded area.

The corresponding photoionization cross sections are shown in Fig. S6 as a function of photon energy. The figure also shows the frequency spectrum of the XUV pulse. As can be seen, all open channels significantly contribute to the total ionization cross section in the whole energy range accessible by the XUV pulse.

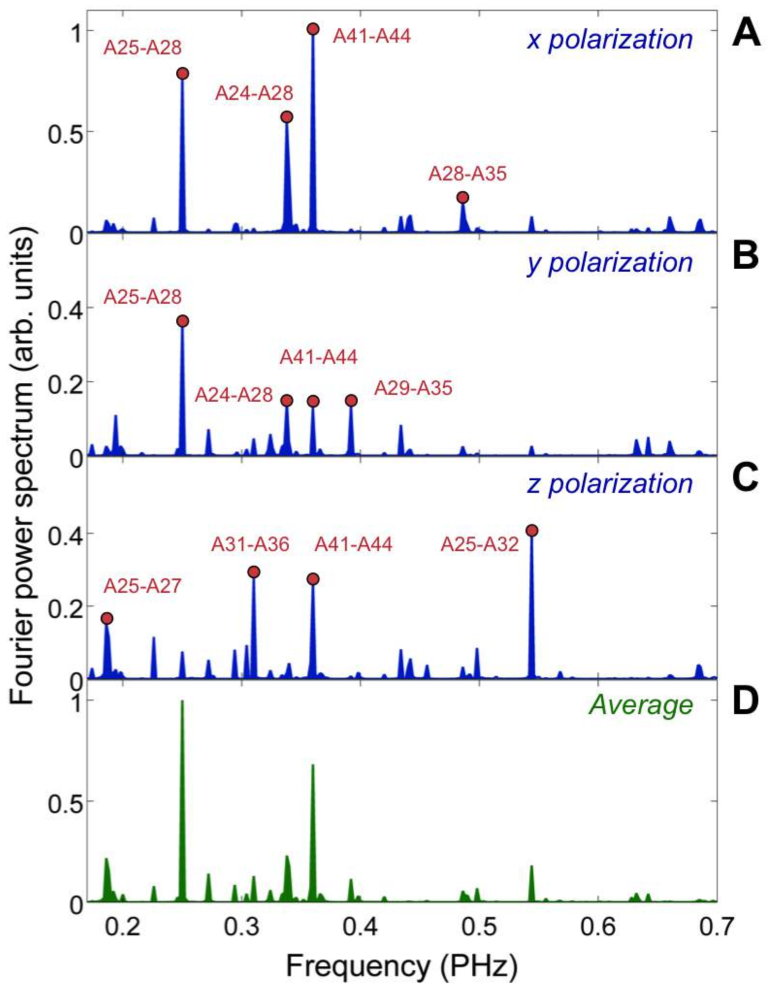


**Fig. S7.**
**Fourier analysis of hole dynamics: dependence on the polarization direction.** Fourier power spectra of the hole density integrated over the amine group for the most abundant conformer of phenylalanine for the three polarization directions defined in Fig. 1 of the manuscript and the average over all polarization directions (randomly oriented molecules). We have also identified the Kohn-Sham orbitals that are responsible for the most important beatings.

Analysis of the observed dynamics

We have evaluated the hole density (Eq. 6) at different values of time, from right after the interaction with the XUV pulse up to 500 fs. We seek to describe the interaction of

linearly polarized light with randomly oriented molecules, so we have considered the three polarization directions *x*, *y* and *z* shown in Fig. 1 of the manuscript.

From the calculated evolution of the hole density it is clear that the largest variations of this density are observed around the amine group (-$NH_2$). In order to perform a more quantitative analysis, we have integrated the hole density around the amine group. Figure S7 shows the results obtained in the case of the most abundant conformer of phenylalanine. The Fourier power spectra of the temporal evolution of the integrated hole densities are displayed for each orientation and the average over polarization direction, assuming randomly oriented molecules.

To better understand the observed dynamics, in Fig. S7 we have identified the Kohn-Sham orbitals that are responsible for the most important beatings. For completeness, the Kohn-Sham molecular orbitals are plotted in Fig. S8. As can be seen, the dominant beatings almost always involve two orbitals with significant density around the amine group, and at least one of these orbitals allows for delocalization over the whole molecule. This is the reason why the hole moves all over the molecule and the dynamics is better observed in the vicinity of the amine group. To further confirm that the observed dynamics can almost be entirely explained in terms of some of the cationic states that are initially populated by the XUV attosecond pulse, we have carried out calculations for the most abundant conformer in which only cationic states resulting from removing an electron from the A24, A25, A28, A29, A31, A32, A35, A36, A41, and A44 orbitals are included in the free propagation of the electronic wave packet.

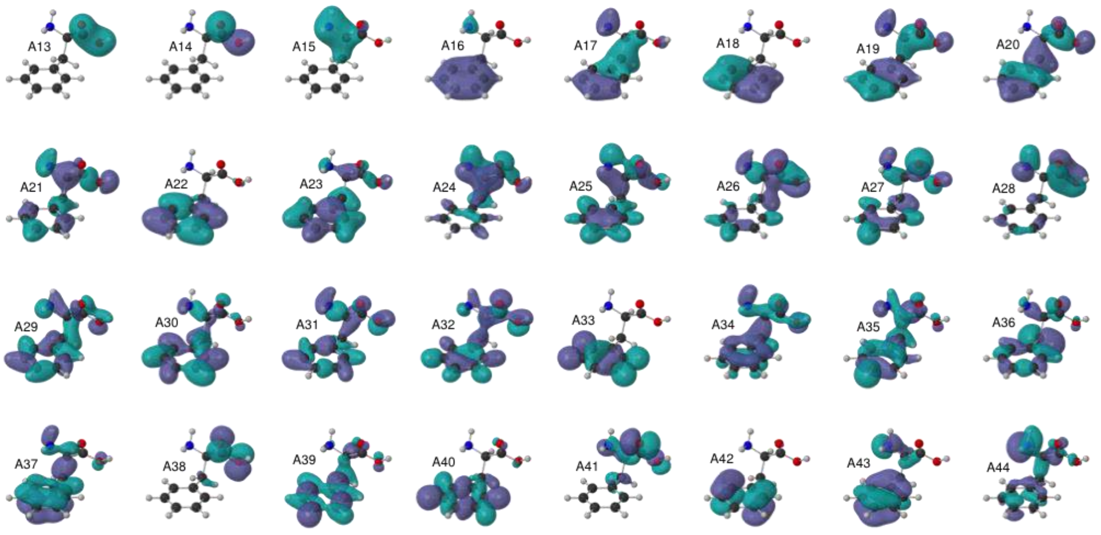


**Fig. S8.**
**Kohn-Sham molecular orbitals.** Calculated Kohn-Sham orbitals of phenylalanine.

Conversely, we have also performed calculations in which all cationic states but the above mentioned ones are included. The results of these two calculations are shown and compared with the full calculations in Fig. S9. As can be seen, the full FT spectrum is almost entirely reproduced by only including the above ten states. In contrast, the dynamics resulting from excluding these states is almost inexistent.

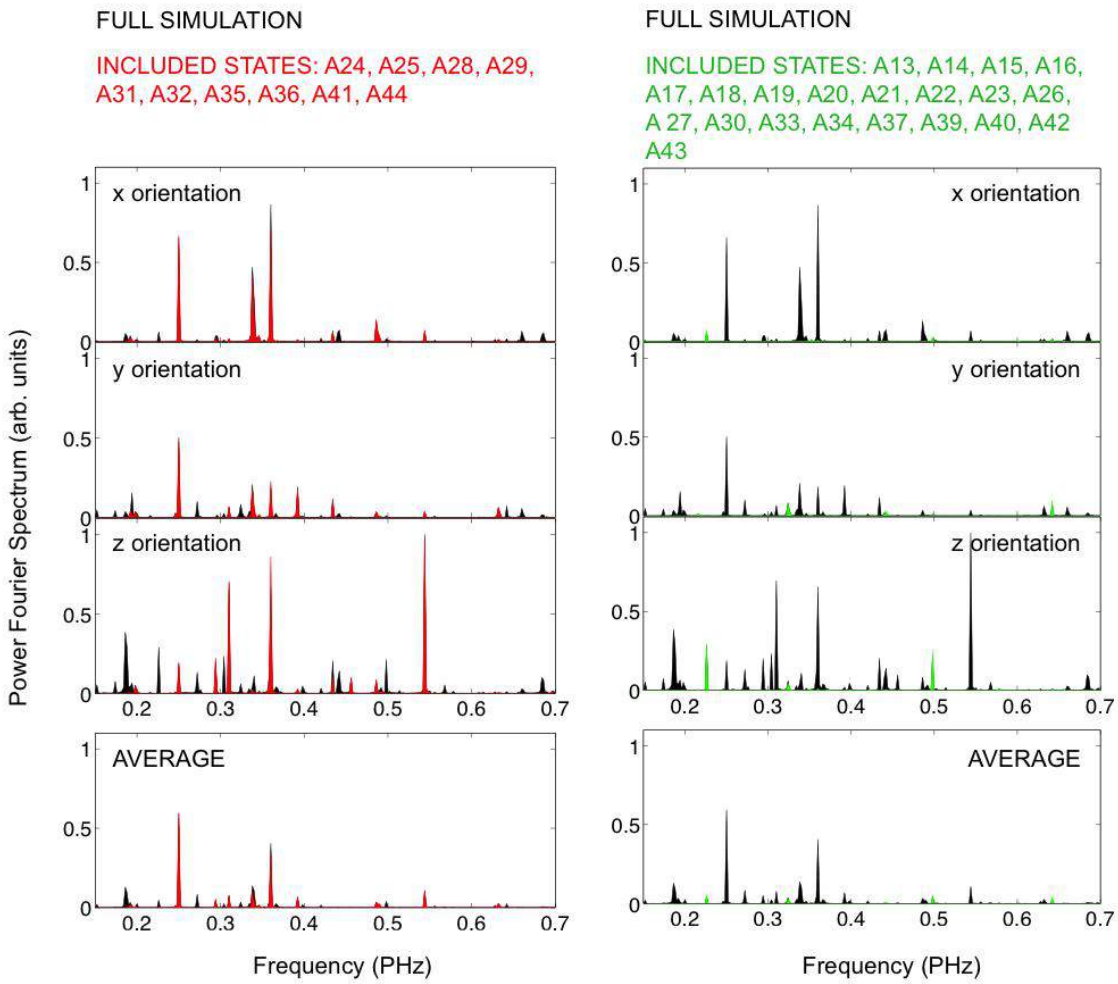


**Fig. S9.**
**Fourier power spectra**. Hole density integrated over the amine group for the most abundant conformer. Black curves: full calculation. Red curves: only cationic states resulting from removing an electron from the A24, A25, A28, A29, A31, A32, A35, A36, A41, and A44 orbitals are included. Green curves: all cationic states but the above mentioned ones are included.

The ultrafast temporal evolution of the wave packet generated by the attosecond pump pulse has also been calculated for the most stable six conformers of phenylalanine. While the precise frequencies of the relevant peaks in the calculated Fourier spectra depend on the particular conformer, the common characteristic is the presence of three dominant groups of Fourier peaks between 0.15 and 0.4 PHz. A thermal average of the various conformers has been calculated, on the basis of the estimated temperature of the phenylalanine molecules (~430 K), by using the ratios calculated by Huang *et al* (*27*), as given in Table S1.
These ratios were obtained by using statistical mechanics methods based on DFT B3LYP quantum chemistry calculations of the geometries, energies, vibrational frequencies and rotational constants of the 37 lowest conformers of phenylalanine.

**Table S1: Equilibrium distributions (%) of Phenylalanine conformers at T = 418 K.** Reported from Ref. (*27*).

| Conformer | Eq. distribution (%) at T = 418 K |
|---|---|
| 1 | 10.6 |
| 2 | 18.1 |
| 3 | 11.1 |
| 4 | 6.0 |
| 5 | 5.7 |
| 6 | 15.4 |

The corresponding Fourier power spectrum is given in Fig. S10B. The peaks around 0.25 PHz and 0.36 PHz, which dominate the corresponding Fourier power spectrum of the most abundant conformer (see Fig. S10A), are clearly visible. Likewise, the low-frequency component at 0.19 PHz is still evident.

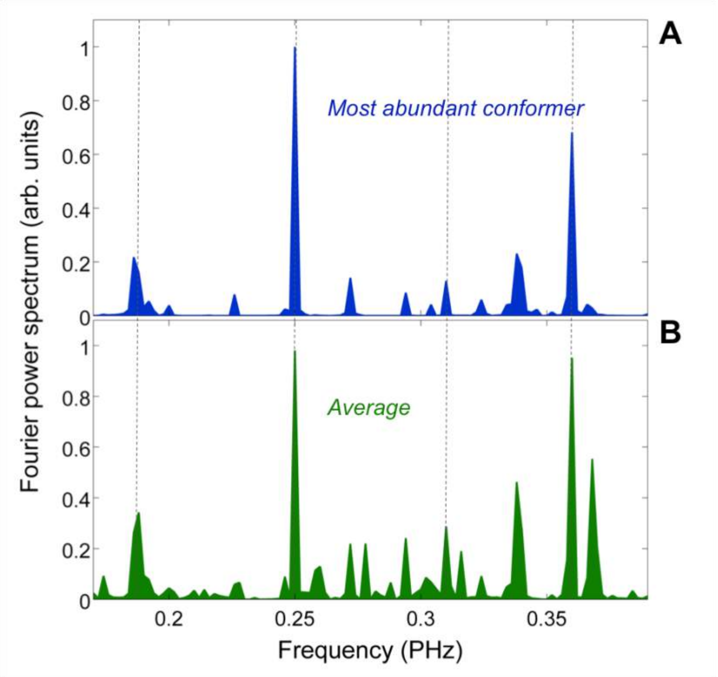


**Fig. S10**.
**Fourier analysis of hole dynamics: role of conformers.** Fourier power spectra of the calculated hole density integrated over amine group: (**A**) most abundant conformer; (**B**) average over the six mostly populated conformers.

We emphasize that the experiment and the calculations probe the specific dynamics generated by the initial pump pulse and go far beyond exclusively providing information about energy spacings between the different quantum states of the phenylalanine molecule. This is dramatically illustrated by Fig. S11, in which the calculated Fourier spectrum corresponding to the most abundant conformer is compared with a similar one containing all possible energy spacings with an equal weight. The dynamics of the

electronic wavepacket generation by the pump pulse is responsible for the fact that only a few beatings are observed. These depend on the dipole matrix elements (i.e., the ionizing transition induced by the XUV attosecond pulse) and the interference between the different amplitudes, which is a direct consequence of the time evolution of the hole density. Moreover, if all six conformers were considered, the bottom panel of Fig. S11 would appear as a quasi-continuum. This is a clear indication that the few beatings that are observed and their relative intensity carry the dynamical information about the ionization step and the subsequent evolution of the hole density.

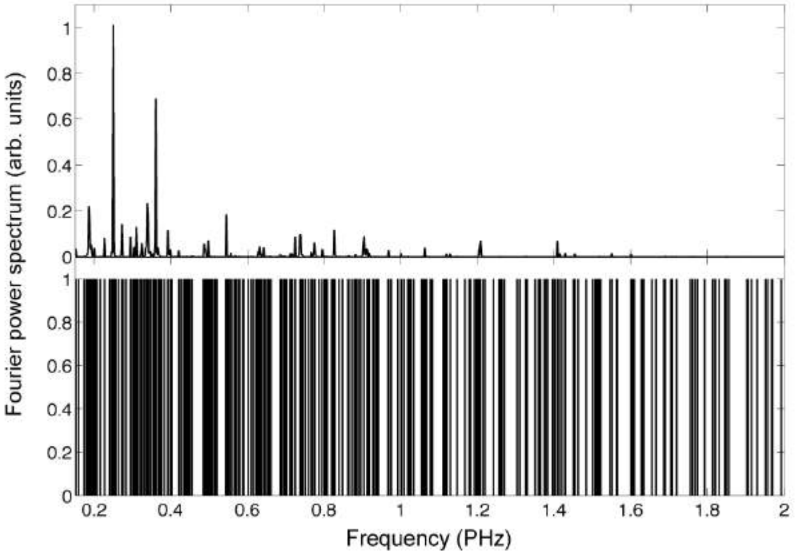


**Fig. S11**.
Fourier power spectra of the calculated hole density integrated over the amine group for the most abundant conformer of phenylalanine. Top: actual calculation. Bottom: results obtained by using an equal weight for all cationic states accessible by the XUV pulse.

Vibrational frequencies of phenylalanine

We have calculated the vibrational frequencies and corresponding vibrational periods of phenylalanine. These have been obtained from standard DFT-B3LYP quantum chemistry calculations. The results are given in Table S2. As can be seen, all the vibrational frequencies (periods) are much smaller (larger) than the frequency (period) of the slowest observed beating. Therefore, one can rule out that the observed beatings are due to vibrational motion.

**Table S2: Vibrational frequencies of phenylalanine.** Frequency ($cm^{-1}$ and PHz) and corresponding periods (fs) of vibrational modes of phenylalanine.

| Mode | Freq. ($cm^{-1}$) | Freq. (PHz) | Period (fs) |
|---|---|---|---|
| 1 | 37.3 | 0.0011 | 894.8 |
| 2 | 45.0 | 0.0013 | 740.7 |
| 3 | 66.8 | 0.0020 | 499.2 |

| | | | |
|---|---|---|---|
| 4 | 104.3 | 0.0031 | 319.9 |
| 5 | 191.5 | 0.0057 | 174.2 |
| 6 | 229.6 | 0.0069 | 145.3 |
| 7 | 248.1 | 0.0074 | 134.5 |
| 8 | 292.9 | 0.0088 | 113.9 |
| 9 | 379.0 | 0.0114 | 88.0 |
| 10 | 408.8 | 0.0123 | 81.6 |
| 11 | 418.2 | 0.0125 | 79.8 |
| 12 | 487.6 | 0.0146 | 68.4 |
| 13 | 493.2 | 0.0148 | 67.6 |
| 14 | 565.8 | 0.0170 | 59.0 |
| 15 | 604.6 | 0.0181 | 55.2 |
| 16 | 635.6 | 0.0191 | 52.5 |
| 17 | 645.0 | 0.0193 | 51.7 |
| 18 | 714.6 | 0.0214 | 46.7 |
| 19 | 733.9 | 0.0220 | 45.5 |
| 20 | 773.4 | 0.0232 | 43.1 |
| 21 | 780.2 | 0.0234 | 42.8 |
| 22 | 855.2 | 0.0256 | 39.0 |
| 23 | 867.3 | 0.0260 | 38.5 |
| 24 | 885.8 | 0.0266 | 37.7 |
| 25 | 922.2 | 0.0276 | 36.2 |
| 26 | 945.6 | 0.0283 | 35.3 |
| 27 | 996.9 | 0.0299 | 33.5 |
| 28 | 1001.0 | 0.0300 | 33.3 |
| 29 | 1008.4 | 0.0302 | 33.1 |
| 30 | 1014.2 | 0.0304 | 32.9 |
| 31 | 1051.5 | 0.0315 | 31.7 |
| 32 | 1105.1 | 0.0331 | 30.2 |
| 33 | 1118.6 | 0.0335 | 29.8 |
| 34 | 1141.6 | 0.0342 | 29.2 |
| 35 | 1177.4 | 0.0353 | 28.3 |
| 36 | 1184.0 | 0.0355 | 28.2 |
| 37 | 1207.1 | 0.0362 | 27.6 |
| 38 | 1218.8 | 0.0365 | 27.4 |
| 39 | 1243.7 | 0.0373 | 26.8 |
| 40 | 1292.8 | 0.0388 | 25.8 |
| 41 | 1330.5 | 0.0399 | 25.1 |
| 42 | 1343.5 | 0.0403 | 24.8 |
| 43 | 1368.9 | 0.0410 | 24.4 |
| 44 | 1377.7 | 0.0413 | 24.2 |
| 45 | 1403.6 | 0.0421 | 23.8 |
| 46 | 1486.9 | 0.0446 | 22.4 |
| 47 | 1487.8 | 0.0446 | 22.4 |
| 48 | 1530.6 | 0.0459 | 21.8 |
| 49 | 1621.4 | 0.0486 | 20.6 |
| 50 | 1643.2 | 0.0493 | 20.3 |
| 51 | 1668.8 | 0.0500 | 20.0 |
| 52 | 1813.3 | 0.0544 | 18.4 |
| 53 | 3024.2 | 0.0907 | 11.0 |
| 54 | 3054.6 | 0.0916 | 10.9 |
| 55 | 3097.8 | 0.0929 | 10.8 |
| 56 | 3154.5 | 0.0946 | 10.6 |
| 57 | 3159.8 | 0.0947 | 10.6 |
| 58 | 3169.5 | 0.0950 | 10.5 |
| 59 | 3176.9 | 0.0952 | 10.5 |

| | | | |
|---|---|---|---|
| 60 | 3187.3 | 0.0956 | 10.5 |
| 61 | 3501.7 | 0.1050 | 9.5 |
| 62 | 3570.7 | 0.1070 | 9.3 |
| 63 | 3754.0 | 0.1125 | 8.9 |

Accuracy of the time-propagation method

To verify the fidelity of our time-propagation method, we have performed theoretical calculations for the glycine molecule, which has been extensively studied by Kuleff *et al*. (*53*). In the latter reference, 2h1p states were explicitly included in the time propagation, so that a direct comparison with their results provides an unambiguous answer about the role played by such states not included in our time propagation scheme. Our results (to be published elsewhere) are in excellent agreement with those of Kuleff *et al*. (*53*). Therefore, in the range of photon energies leading to the cationic states relevant for the observed dynamics, we can safely conclude that 2h1p states do not play a significant role.

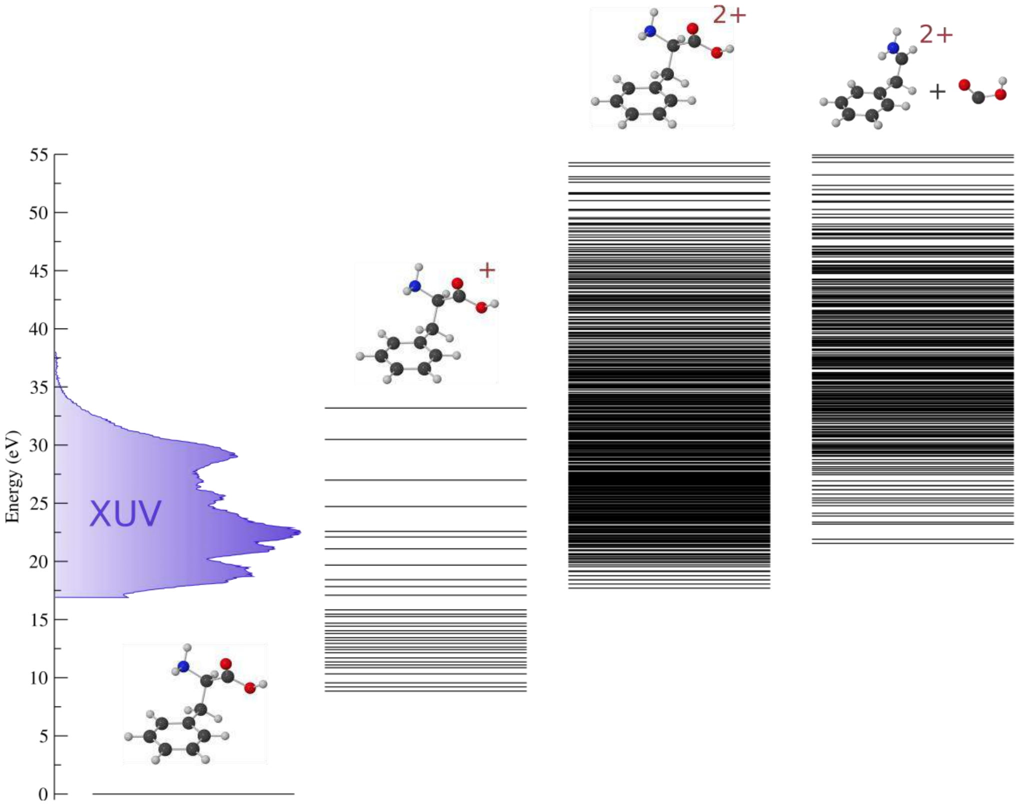


**Fig. S12.**
Energy level diagram containing all the states of singly charged phenylalanine created by the XUV pulse, all the states of doubly-charged phenylalanine and those for the system immonium$^{++}$ + COOH.

Possible probe mechanisms
Figure S12 shows an energy-level diagram with all the states of singly charged phenylalanine ($P^+$) created by the XUV pulse, all the states of doubly-charged phenylalanine ($P^{++}$) and those for the system (immonium$^{++}$ + COOH) (for short $I^{++}$). The

energies of the latter two systems have been generated by removing electrons from all molecular orbitals of $P^+$ and immonium+, respectively. As can be seen, one can go from a highly excited state of $P^+$ to the lowest states of $P^{++}$ or $I^{++}$ by absorbing just a few VIS/NIR photons (photon energy around 1.77 eV). Of course, one cannot know how likely this transition will be, but one can unambiguously say that the process only requires absorption of very few VIS/NIR photons. Even if these transitions were unlikely, e.g., due to unfavorable overlap between initial and final orbitals, the transition should be much more likely than others involving many photons even with favorable overlap.

**Movie S1**

The movie depicts the calculated temporal evolution of the relative variation of the hole density with respect to its time-averaged value  for the most abundant conformer of phenylalanine. Iso-surfaces of the relative hole density are shown for cutoff values of $+10^{-4}$ a.u. (yellow) and $-10^{-4}$ (purple). Time is referred to the end of the XUV pulse.

## References and Notes


1. F. Krausz, M. Ivanov, Attosecond physics. *Rev. Mod. Phys.* **81**, 163–234 (2009). doi:10.1103/RevModPhys.81.163

2. M. Drescher, M. Hentschel, R. Kienberger, M. Uiberacker, V. Yakovlev, A. Scrinzi, T. Westerwalbesloh, U. Kleineberg, U. Heinzmann, F. Krausz, Time-resolved atomic inner-shell spectroscopy. *Nature* **419**, 803–807 (2002). Medline doi:10.1038/nature01143

3. M. Uiberacker, T. Uphues, M. Schultze, A. J. Verhoef, V. Yakovlev, M. F. Kling, J. Rauschenberger, N. M. Kabachnik, H. Schröder, M. Lezius, K. L. Kompa, H. G. Muller, M. J. Vrakking, S. Hendel, U. Kleineberg, U. Heinzmann, M. Drescher, F. Krausz, Attosecond real-time observation of electron tunnelling in atoms. *Nature* **446**, 627–632 (2007). Medline doi:10.1038/nature05648

4. M. Schultze, M. Fiess, N. Karpowicz, J. Gagnon, M. Korbman, M. Hofstetter, S. Neppl, A. L. Cavalieri, Y. Komninos, T. Mercouris, C. A. Nicolaides, R. Pazourek, S. Nagele, J. Feist, J. Burgdörfer, A. M. Azzeer, R. Ernstorfer, R. Kienberger, U. Kleineberg, E. Goulielmakis, F. Krausz, V. S. Yakovlev, Delay in photoemission. *Science* **328**, 1658–1662 (2010). Medline doi:10.1126/science.1189401

5. K. Klünder, J. M. Dahlström, M. Gisselbrecht, T. Fordell, M. Swoboda, D. Guénot, P. Johnsson, J. Caillat, J. Mauritsson, A. Maquet, R. Taïeb, A. L'Huillier, Probing single-photon ionization on the attosecond time scale. *Phys. Rev. Lett.* **106**, 143002 (2011). Medline doi:10.1103/PhysRevLett.106.143002

6. E. Goulielmakis, Z. H. Loh, A. Wirth, R. Santra, N. Rohringer, V. S. Yakovlev, S. Zherebtsov, T. Pfeifer, A. M. Azzeer, M. F. Kling, S. R. Leone, F. Krausz, Real-time observation of valence electron motion. *Nature* **466**, 739–743 (2010). Medline doi:10.1038/nature09212

7. A. L. Cavalieri, N. Müller, T. Uphues, V. S. Yakovlev, A. Baltuska, B. Horvath, B. Schmidt, L. Blümel, R. Holzwarth, S. Hendel, M. Drescher, U. Kleineberg, P. M. Echenique, R. Kienberger, F. Krausz, U. Heinzmann, Attosecond spectroscopy in condensed matter. *Nature* **449**, 1029–1032 (2007). Medline doi:10.1038/nature06229

8. A. Schiffrin, T. Paasch-Colberg, N. Karpowicz, V. Apalkov, D. Gerster, S. Mühlbrandt, M. Korbman, J. Reichert, M. Schultze, S. Holzner, J. V. Barth, R. Kienberger, R. Ernstorfer, V. S. Yakovlev, M. I. Stockman, F. Krausz, Optical-field-induced current in dielectrics. *Nature* **493**, 70–74 (2013). Medline doi:10.1038/nature11567

9. F. Lépine, M. Y. Ivanov, M. J. J. Vrakking, Attosecond molecular dynamics: Fact or fiction? *Nat. Photonics* **8**, 195–204 (2014). doi:10.1038/nphoton.2014.25

10. G. Sansone, F. Kelkensberg, J. F. Pérez-Torres, F. Morales, M. F. Kling, W. Siu, O. Ghafur, P. Johnsson, M. Swoboda, E. Benedetti, F. Ferrari, F. Lépine, J. L. Sanz-Vicario, S. Zherebtsov, I. Znakovskaya, A. L'huillier, M. Y. Ivanov, M. Nisoli, F. Martín, M. J. Vrakking, Electron localization following attosecond molecular photoionization. *Nature* **465**, 763–766 (2010). Medline doi:10.1038/nature09084

11. F. Kelkensberg, W. Siu, J. F. Pérez-Torres, F. Morales, G. Gademann, A. Rouzée, P. Johnsson, M. Lucchini, F. Calegari, J. L. Sanz-Vicario, F. Martín, M. J. Vrakking,

Attosecond control in photoionization of hydrogen molecules. *Phys. Rev. Lett.* **107**, 043002 (2011). Medline doi:10.1103/PhysRevLett.107.043002

12. W. Siu, F. Kelkensberg, G. Gademann, A. Rouzée, P. Johnsson, D. Dowek, M. Lucchini, F. Calegari, U. De Giovannini, A. Rubio, R. R. Lucchese, H. Kono, F. Lépine, M. J. J. Vrakking, Attosecond control of dissociative ionization of $O_2$ molecules. *Phys. Rev. A* **84**, 063412 (2011). doi:10.1103/PhysRevA.84.063412

13. P. Ranitovic, C. W. Hogle, P. Rivière, A. Palacios, X. M. Tong, N. Toshima, A. González-Castrillo, L. Martin, F. Martín, M. M. Murnane, H. Kapteyn, Attosecond vacuum UV coherent control of molecular dynamics. *Proc. Natl. Acad. Sci. U.S.A.* **111**, 912–917 (2014). Medline doi:10.1073/pnas.1321999111

14. L. Belshaw, F. Calegari, M. J. Duffy, A. Trabattoni, L. Poletto, M. Nisoli, J. B. Greenwood, Observation of ultrafast charge migration in an amino acid. *J. Phys. Chem. Lett.* **3**, 3751–3754 (2012). doi:10.1021/jz3016028

15. F. Remacle, R. D. Levine, An electronic time scale in chemistry. *Proc. Natl. Acad. Sci. U.S.A.* **103**, 6793–6798 (2006). Medline doi:10.1073/pnas.0601855103

16. L. S. Cederbaum, J. Zobeley, Ultrafast charge migration by electron correlation. *Chem. Phys. Lett.* **307**, 205–210 (1999). doi:10.1016/S0009-2614(99)00508-4

17. H. Hennig, J. Breidbach, L. S. Cederbaum, Electron correlation as the driving force for charge transfer: Charge migration following ionization in N-methyl acetamide. *J. Phys. Chem. A* **109**, 409–414 (2005). Medline doi:10.1021/jp046232s

18. J. Breidbach, L. S. Cederbaum, Universal attosecond response to the removal of an electron. *Phys. Rev. Lett.* **94**, 033901 (2005). Medline doi:10.1103/PhysRevLett.94.033901

19. J. Breidbach, L. S. Cederbaum, Migration of holes: Formalism, mechanisms, and illustrative applications. *J. Chem. Phys.* **118**, 3983 (2003). doi:10.1063/1.1540618

20. R. Weinkauf, P. Schanen, D. Yang, S. Soukara, E. W. Schlag, Elementary processes in peptides: electron mobility and dissociation in peptide cations in the gas phase. *J. Phys. Chem.* **99**, 11255–11265 (1995). doi:10.1021/j100028a029

21. R. Weinkauf, P. Schanen, A. Metsala, E. W. Schlag, M. Bürgle, H. Kessler, Highly efficient charge transfer in peptide cations in the gas phase: threshold effects and mechanism. *J. Phys. Chem.* **100**, 18567–18585 (1996). doi:10.1021/jp960926m

22. J. Wals, H. H. Fielding, J. F. Christian, L. C. Snoek, W. J. van der Zande, H. van Linden van den Heuvell, Observation of Rydberg wave packet dynamics in a Coulombic and magnetic field. *Phys. Rev. Lett.* **72**, 3783–3786 (1994). Medline doi:10.1103/PhysRevLett.72.3783

23. C. R. Calvert, L. Belshaw, M. J. Duffy, O. Kelly, R. B. King, A. G. Smyth, T. J. Kelly, J. T. Costello, D. J. Timson, W. A. Bryan, T. Kierspel, P. Rice, I. C. Turcu, C. M. Cacho, E. Springate, I. D. Williams, J. B. Greenwood, LIAD-fs scheme for studies of ultrafast laser interactions with gas phase biomolecules. *Phys. Chem. Chem. Phys.* **14**, 6289–6297 (2012). Medline doi:10.1039/c2cp23840c

24. S. Lünnemann, A. I. Kuleff, L. S. Cederbaum, Ultrafast charge migration in 2-phenylethyl-N,N-dimethylamine. *Chem. Phys. Lett.* **450**, 232–235 (2008). doi:10.1016/j.cplett.2007.11.031

25. D. Mendive-Tapia, M. Vacher, M. J. Bearpark, M. A. Robb, Coupled electron-nuclear dynamics: Charge migration and charge transfer initiated near a conical intersection. *J. Chem. Phys.* **139**, 044110 (2013). Medline doi:10.1063/1.4815914

26. A. I. Kuleff, L. S. Cederbaum, Charge migration in different conformers of glycine: The role of nuclear geometry. *Chem. Phys.* **338**, 320–328 (2007). doi:10.1016/j.chemphys.2007.04.012

27. H. Z. Huang, W. Yu, Z. Lin, Exploration of the full conformational landscapes of gaseous aromatic amino acid phenylalanine: An ab initio study. *J. Mol. Struct. THEOCHEM* **758**, 195–202 (2006). doi:10.1016/j.theochem.2005.10.043

28. D. Toffoli, M. Stener, G. Fronzoni, P. Decleva, Convergence of the multicenter B-spline DFT approach for the continuum. *Chem. Phys.* **276**, 25–43 (2002). doi:10.1016/S0301-0104(01)00549-3

29. E. Plésiat, P. Decleva, F. Martín, Vibrational branching ratios in the photoelectron spectra of N2 and CO: Interference and diffraction effects. *Phys. Chem. Chem. Phys.* **14**, 10853–10871 (2012). Medline doi:10.1039/c2cp40693d

30. S. E. Canton, E. Plésiat, J. D. Bozek, B. S. Rude, P. Decleva, F. Martín, Direct observation of Young's double-slit interferences in vibrationally resolved photoionization of diatomic molecules. *Proc. Natl. Acad. Sci. U.S.A.* **108**, 7302–7306 (2011). doi:10.1073/pnas.1018534108

31. O. Plekan, V. Feyer, R. Richter, M. Coreno, K. C. Prince, Valence photoionization and photofragmentation of aromatic amino acids. *Mol. Phys.* **106**, 1143–1153 (2008). doi:10.1080/00268970801974875

32. M. Nisoli, S. De Silvestri, O. Svelto, Generation of high energy 10 fs pulses by a new pulse compression technique. *Appl. Phys. Lett.* **68**, 2793 (1996). doi:10.1063/1.116609

33. A. Suda, M. Hatayama, K. Nagasaka, K. Midorikawa, Generation of sub-10-fs, 5-mJ-optical pulses using a hollow fiber with a pressure gradient. *Appl. Phys. Lett.* **86**, 111116 (2005). doi:10.1063/1.1883706

34. T. Oksenhendler, S. Coudreau, N. Forget, V. Crozatier, S. Grabielle, R. Herzog, O. Gobert, D. Kaplan, Self-referenced spectral interferometry. *Appl. Phys. B* **99**, 7–12 (2010). doi:10.1007/s00340-010-3916-y

35. F. Ferrari, F. Calegari, M. Lucchini, C. Vozzi, S. Stagira, G. Sansone, M. Nisoli, High-energy isolated attosecond pulses generated by above-saturation few-cycle fields. *Nature Phot.* **4**, 875–879 (2010). doi:10.1038/nphoton.2010.250

36. Y. Mairesse, F. Quéré, Frequency-resolved optical gating for complete reconstruction of attosecond bursts. *Phys. Rev. A* **71**, 011401(R) (2005). doi:10.1103/PhysRevA.71.011401

37. G. Sansone, E. Benedetti, F. Calegari, C. Vozzi, L. Avaldi, R. Flammini, L. Poletto, P. Villoresi, C. Altucci, R. Velotta, S. Stagira, S. De Silvestri, M. Nisoli, Isolated single-

cycle attosecond pulses. *Science* **314**, 443–446 (2006). Medline doi:10.1126/science.1132838

38. L. Poletto, S. Bonora, M. Pascolini, P. Villoresi, Instrumentation for analysis and utilization of extreme-ultraviolet and soft x-ray high-order harmonics. *Rev. Sci. Instrum.* **75**, 4413 (2004). doi:10.1063/1.1784563
39. S. Boyden, J. Zhang, Temperature and wavelength-dependent spectral absorptivities of metallic materials in the infrared. *J. Therm. Heat Transfer* **20**, 9–15 (2006). doi:10.2514/1.15518
40. F. Gaie-Levrel, G. A. Garcia, M. Schwell, L. Nahon, VUV state-selected photoionization of thermally-desorbed biomolecules by coupling an aerosol source to an imaging photoelectron/photoion coincidence spectrometer: Case of the amino acids tryptophan and phenylalanine. *Phys. Chem. Chem. Phys.* **13**, 7024–7036 (2011). Medline doi:10.1039/c0cp02798g
41. M. Stener, P. Bolognesi, M. Coreno, P. O'Keeffe, V. Feyer, G. Fronzoni, P. Decleva, L. Avaldi, A. Kivimäki, Photoabsorption and S 2p photoionization of the SF6 molecule: Resonances in the excitation energy range of 200-280 eV. *J. Chem. Phys.* **134**, 174311 (2011). Medline doi:10.1063/1.3583815
42. D. Catone, M. Stener, P. Decleva, G. Contini, N. Zema, T. Prosperi, V. Feyer, K. C. Prince, S. Turchini, Resonant circular dichroism of chiral metal-organic complex. *Phys. Rev. Lett.* **108**, 083001 (2012). Medline doi:10.1103/PhysRevLett.108.083001
43. L. Argenti, T. D. Thomas, E. Plésiat, X.-J. Liu, C. Miron, T. Lischke, G. Prümper, K. Sakai, T. Ouchi, R. Püttner, V. Sekushin, T. Tanaka, M. Hoshino, H. Tanaka, P. Decleva, K. Ueda, F. Martín, Double-slit experiment with a polyatomic molecule: Vibrationally resolved C 1s photoelectron spectra of acetylene. *New J. Phys.* **14**, 033012 (2012). doi:10.1088/1367-2630/14/3/033012
44. S. Turchini, D. Catone, N. Zema, G. Contini, T. Prosperi, P. Decleva, M. Stener, F. Rondino, S. Piccirillo, K. C. Prince, M. Speranza, Conformational sensitivity in photoelectron circular dichroism of 3-methylcyclopentanone. *ChemPhysChem* **14**, 1723–1732 (2013). Medline doi:10.1002/cphc.201200975
45. R. K. Kushawaha, M. Patanen, R. Guillemin, L. Journel, C. Miron, M. Simon, M. N. Piancastelli, C. Skates, P. Decleva, From double-slit interference to structural information in simple hydrocarbons. *Proc. Natl. Acad. Sci. U.S.A.* **110**, 15201–15206 (2013). Medline doi:10.1073/pnas.1306697110
46. K. Ueda, C. Miron, E. Plésiat, L. Argenti, M. Patanen, K. Kooser, D. Ayuso, S. Mondal, M. Kimura, K. Sakai, O. Travnikova, A. Palacios, P. Decleva, E. Kukk, F. Martín, Intramolecular photoelectron diffraction in the gas phase. *J. Chem. Phys.* **139**, 124306 (2013). Medline doi:10.1063/1.4820814
47. D. M. P. Holland, D. A. Shaw, S. Coriani, M. Stener, P. Decleva, A study of the valence shell electronic states of pyridazine by photoabsorption spectroscopy and time-dependent density functional theory calculations. *J. Phys. At. Mol. Opt. Phys.* **46**, 175103 (2013). doi:10.1088/0953-4075/46/17/175103

48. E. Plésiat, P. Decleva, F. Martín, Relationship between polarization-averaged molecular-frame photoelectron angular distributions and geometry. *Phys. Rev. A* **88**, 063409 (2013). doi:10.1103/PhysRevA.88.063409

49. R. Boll, D. Anielski, C. Bostedt, J. Bozek, L. Christensen, R. Coffee, S. De, P. Decleva, S. Epp, B. Erk, L. Foucar, F. Krasniqi, J. Küpper, A. Rouzée, B. Rudek, A. Rudenko, S. Schorb, H. Stapelfeldt, M. Stener, S. Stern, S. Techert, S. Trippel, M. Vrakking, J. Ullrich, D. Rolles, Femtosecond photoelectron diffraction on laser-aligned molecules: Towards time-resolved imaging of molecular structure. *Phys. Rev. A* **88**, 061402 (2013). doi:10.1103/PhysRevA.88.061402

50. M. Stener, P. Decleva, T. Mizuno, H. Yoshida, A. Yagishita, Off-resonance photoemission dynamics studied by recoil frame F1s and C1s photoelectron angular distributions of $CH_3F$. *J. Chem. Phys.* **140**, 044305 (2014). doi:10.1063/1.4862267

51. K. Blum, *Density Matrix Theory and Applications* (Plenum, New York, 1996).

52. N. Rohringer, R. Santra, Multichannel coherence in strong-field ionization. *Phys. Rev. A* **79**, 053402 (2009). doi:10.1103/PhysRevA.79.053402

53. A. I. Kuleff, J. Breidbach, L. S. Cederbaum, Multielectron wave-packet propagation: General theory and application. *J. Chem. Phys.* **123**, 044111 (2005). Medline doi:10.1063/1.1961341
